# Supplementary material for: Bongard in Wonderland: Visual Puzzles that Still Make AI Go Mad?
Source: arXiv:2410.19546 source file (2025-07-12)
Supplement: Supplementary file 1 [file solved_bps_vlms_vs_humans_transposed.tex]

\begin{table}[t]
    \centering
    \caption{Results for each model across individual Bongard Problems, converted into percentages, compared to the results of 13 humans reported in \cite{depeweg2018solving}. Each model was prompted \(X\) times, and the number of correct responses is reported as a fraction of \(X\).}
    \label{tab:models_vs_problems_percentage}
    \resizebox{1.05\columnwidth}{!}{%
\begin{tabular}{lllllllllllllllllllllllllllllllllllllll}
\toprule
BP\# & 1 & 2 & 3 & 4 & 6 & 7 & 8 & 9 & 11 & 12 & 21 & 22 & 23 & 24 & 25 & 26 & 27 & 28 & 29 & 34 & 35 & 36 & 37 & 38 & 39 & 40 & 41 & 42 & 47 & 48 & 49 \\
\midrule
\textbf{GPT-4o} & \cellcolor{PineGreen!25}1.0 & 0.08 & \cellcolor{PineGreen!25}1.0 & 0.0 & \cellcolor{PineGreen!25}1.0 & 0.54 & 0.0 & 0.0 & 0.0 & 0.15 & 0.0 & 0.0 & 0.27 & 0.0 & 0.64 & 0.0 & 0.0 & 0.0 & 0.0 & 0.0 & 0.0 & 0.0 & 0.0 & 0.0 & 0.0 & 0.0 & 0.0 & 0.0 & \cellcolor{PineGreen!25}1.0 & 0.0 & 0.0 \\
\textbf{Claude} & \cellcolor{Green!25}0.92 & 0.31 & \cellcolor{PineGreen!25}1.0 & 0.08 & 0.38 & 0.62 & 0.0 & 0.15 & 0.0 & 0.0 & 0.33 & 0.0 & 1.0 & 0.18 & 0.09 & 0.0 & 0.0 & 0.0 & 0.0 & 0.0 & 0.11 & 0.11 & 0.0 & 0.38 & 0.12 & 0.0 & 0.0 & 0.0 & 0.5 & 0.0 & 0.0 \\
\textbf{Gemini} & \cellcolor{Green!25}0.92 & 0.0 & 0.38 & 0.0 & 0.0 & 0.0 & 0.0 & 0.08 & 0.0 & 0.0 & 0.0 & 0.0 & 0.27 & 0.0 & 0.0 & 0.0 & 0.0 & 0.0 & 0.0 & 0.0 & 0.11 & 0.0 & 0.0 & 0.0 & 0.0 & 0.0 & 0.0 & 0.0 & 0.83 & 0.0 & 0.0 \\
\textbf{LLaVA 1.6} & 0.0 & 0.0 & 0.0 & 0.0 & 0.08 & 0.0 & 0.0 & 0.0 & 0.0 & 0.0 & 0.0 & 0.0 & 0.18 & 0.0 & 0.18 & 0.0 & 0.0 & 0.0 & 0.0 & 0.0 & 0.0 & 0.0 & 0.0 & 0.0 & 0.0 & 0.0 & 0.0 & 0.0 & 0.0 & 0.0 & 0.0 \\
\textbf{Humans} & \cellcolor{PineGreen!25}1.0 & \cellcolor{Green!25}0.85 & \cellcolor{PineGreen!25}1.0 & 0.23 & \cellcolor{Green!25}0.92 & \cellcolor{PineGreen!25}1.0 & \cellcolor{PineGreen!25}1.0 & \cellcolor{Green!25}0.92 & 0.62 & 0.54 & \cellcolor{Green!25}0.83 & \cellcolor{Green!25}0.92 & \cellcolor{PineGreen!25}1.0 & \cellcolor{Green!25}0.91 & \cellcolor{Green!25}0.82 & \cellcolor{Green!25}0.9 & \cellcolor{Green!25}0.8 & 0.4 & \cellcolor{Green!25}0.7 & \cellcolor{PineGreen!25}1.0 & \cellcolor{PineGreen!25}1.0 & \cellcolor{PineGreen!25}1.0 & 0.38 & \cellcolor{Green!25}0.75 & \cellcolor{PineGreen!25}1.0 & \cellcolor{PineGreen!25}1.0 & \cellcolor{PineGreen!25}1.0 & \cellcolor{PineGreen!25}1.0 & \cellcolor{PineGreen!25}1.0 & \cellcolor{PineGreen!25}1.0 \\
\midrule
\textbf{All solved} & 4 & 2 & 0 & 0 & 15 \\
\textbf{2/3 solved} & 4 & 3 & 2 & 0 & 26 \\
\bottomrule
\end{tabular}
}
\end{table}
