# Supplementary material for: Bongard in Wonderland: Visual Puzzles that Still Make AI Go Mad?
Source: arXiv:2410.19546 source file (2025-07-12)
Supplement: Supplementary file 2 [file prompt_count.tex]

% \begin{lstlisting}[language={}, label=lst:count_prompt, basicstyle=\tiny, caption=Prompt for concepts of BP\#29.]
\begin{listing}[h]
\caption{Prompt for concepts of BP\#29}
\label{lst:count_prompt}
\begin{minted}[mathescape,
               linenos,
               numbersep=5pt,
               gobble=0,
               frame=lines,
               framesep=2mm,
               fontsize=\footnotesize,
               breaksymbolleft={},
               tabsize=2,breaklines]{text}
Your task is to determine if the number of objects inside a big shape is bigger than the number of objects outside of it in a 2D black and white diagram. 
The given diagram shows a big shape that can contain smaller shapes inside it. There can also be other small shapes outside of the big shape. Is the number of shapes inside or outside the big shape higher?

Please decide carefully. Take a deep breath and think step-by-step. Give your answer in the following format:
```
answer = {
    "more shapes": <your answer>
}
```
where <your answer> can be either "inside" if the number of shapes inside the big shape is higher or "outside" if the number of shapes outside the big shape is higher.
\end{minted}
\end{listing}
