# Supplementary material for: Bongard in Wonderland: Visual Puzzles that Still Make AI Go Mad?
Source: arXiv:2410.19546 source file (2025-07-12)
Supplement: Supplementary file 3 [file prompt_pinch.tex]

% \begin{lstlisting}[language={}, label=lst:count_prompt, caption=Prompt for concepts of BP\#29.]
\begin{listing}[h]
\caption{Prompt for concepts of BP\#19.}
\label{lst:pinch_prompt}
\begin{minted}[mathescape,
               linenos,
               numbersep=5pt,
               gobble=0,
               frame=lines,
               framesep=2mm,
               fontsize=\footnotesize,
               breaksymbolleft={},
               tabsize=2,breaklines]{text}

Your task is to determine the orientation of a pinch or neck in a 2D black and white diagram. 
The given diagram shows a shape that has a pinch in the middle. The pinch connects the both ends of the shapes and can be interpreted as a bridge as well. Which orientation does this pinch have, horizontal or vertical?

Please decide carefully. Take a deep breath and think step-by-step. Give your answer in the following format:
```
answer = {
    "orientation": <your answer>
}
```
where <your answer> can be either "horizontal" if the bridge is aligned horizontal or "vertical" if the bridge is aligned vertical.
\end{minted}
\end{listing}
