# Supplementary material for: Bongard in Wonderland: Visual Puzzles that Still Make AI Go Mad?
Source: arXiv:2410.19546 source file (2025-07-12)
Supplement: Supplementary file 4 [file prompt_triangle.tex]

% \begin{lstlisting}[language={}, label=lst:triangle_prompt, basicstyle=\tiny, caption=Prompt for concepts of BP\#36.]

\begin{listing}[h]
\caption{Prompt for concepts of BP\#36.}
\label{lst:triangle_prompt}
\begin{minted}[mathescape,
               linenos,
               numbersep=5pt,
               gobble=0,
               frame=lines,
               framesep=2mm,
               fontsize=\footnotesize,
               breaksymbolleft={},
               tabsize=2,breaklines]{text}

Your task is to determine the relative position of two objects in a 2D black and white diagram. 
The given diagram shows a triangle and a circle. Which of the shapes is located above the other, i.e., has a higher y-value than the other?

Please decide carefully. Take a deep breath and think step-by-step. Give your answer in the following format:
```
answer = {
    "shape": <your answer>
}
```
where <your answer> can be either "triangle" if the triangle is above the circle or "circle" if the circle is above the triangle.
\end{minted}
\end{listing}
