# Supplementary material for: Bongard in Wonderland: Visual Puzzles that Still Make AI Go Mad?
Source: arXiv:2410.19546 source file (2025-07-12)
Supplement: Supplementary file 5 [file solved_bps_vlms_vs_humans_aggregated.tex]

% \begin{table*}[t]
%     \centering

%     \caption{[DRAFT] Results of each VLM on the individual Bongard Problems compared to the results of humans. mean of the correct responses per BP is reported. \textit{Cf.} \autoref{tab:vlms_vs_humans} for performance on single BPs.}
%     \label{tab:vlms_vs_humans_agg}
    
% \resizebox{0.95\linewidth}{!}{%

% \begin{tabular}{llllllllll}
% \toprule
%  & humans & o1 & gpt-4o & claude-3-5-sonnet-20241022 & gemini-2.0-flash-exp & gemini & LlavaOnevision & Qwen2VL & InternVL2_5 \\
% \midrule
% size & 43.33 & 61.11 & 16.67 & 27.78 & 5.55 & 0.00 & 0.00 & 0.00 & 0.00 \\
% concept & 46.83 & 70.00 & 45.56 & 48.89 & 38.89 & 12.22 & 14.44 & 20.00 & 27.78 \\
% number & 33.33 & 37.78 & 8.89 & 22.22 & 17.78 & 2.22 & 0.00 & 15.56 & 8.89 \\
% spatial & 40.61 & 17.07 & 8.13 & 13.01 & 12.20 & 0.81 & 0.81 & 5.69 & 6.50 \\
% same & 44.29 & 28.57 & 19.05 & 28.57 & 23.81 & 0.00 & 0.00 & 0.00 & 9.52 \\
% \midrule
% all & 41.82 & 39.73 & 20.88 & 27.27 & 21.55 & 4.38 & 4.71 & 10.77 & 13.13 \\
% \bottomrule
% \end{tabular}


% existence & \textbf{\gradient{93.64}} & \gradient{33.33} & \gradient{38.46} & \gradient{30.77} & \gradient{0.00} & \gradient{0.00}\\
% size & \textbf{\gradient{86.92}} & \gradient{1.54} & \gradient{21.54} & \gradient{0.00} & \gradient{0.00} & \gradient{0.00} \\
% concept & \textbf{\gradient{72.13}} & \gradient{39.56} & \gradient{25.27} & \gradient{6.59} & \gradient{3.30} & \gradient{4.40} \\
% number & \textbf{\gradient{72.50}} & \gradient{7.69} & \gradient{25.00} & \gradient{5.77} & \gradient{3.85} & \gradient{0.00}\\
% spatial & \textbf{\gradient{93.75}} & \gradient{10.00} & \gradient{8.46} & \gradient{7.69} & \gradient{0.00} & \gradient{0.00} \\ \midrule
% All & \textbf{\gradient{84.41}} & \gradient{17.77} & \gradient{20.16} & \gradient{8.22} & \gradient{1.33} & \gradient{1.06}\\

% \vspace{2ex}

% }

% \end{table*}
